# Supplementary material for: Cyclic Contrastive Knowledge Transfer for Open-Vocabulary Object Detection
Source: arXiv:2503.11005 source file (2025-04-02)
Supplement: Supplementary file 1 [file appendix_pseudo_codes.tex]

\section{Appendix A1}

\definecolor{customgreen}{rgb}{0.1, 0.5, 0.1} 

\lstset{
    basicstyle=\ttfamily\small,           
    keywordstyle=\color{black}\ttfamily,  
    commentstyle=\color{customgreen}\ttfamily,  
    stringstyle=\color{black}\ttfamily,   
    showstringspaces=false,               
    columns=fullflexible,                 
    numbers=left,                         
    numberstyle=\tiny\color{gray},        
    breaklines=true,                      
    frame=lines,             
    language=Python,                      
    morekeywords={f, transformer, bbox_head, feature_head, hungarian_matcher,
                  semantic_features, regional_guidance, x, targets, query_embeds,
                  gt_boxes, gt_labels, srcs, hs, pred_boxes, pred_embeds,
                  indices, bbox_loss, L1, GiOU, similarity_score, target_positives_map,
                  Contras, loss}          
}

\begin{lstlisting}[caption={Pseudocode for our method in PyTorch-like style}]
# f: Backbone feature extractor
# transformer: Transformer encoder-decoder
# bbox_head: MLP for bounding box prediction
# feature_head: Projection Layer for contrastive feature distillation and class prediction
# hungarian_matcher: Hungarian matching algorithm

# semantic_features: Categories semantic features encoded by CLIP text encoder
# regional_guidance: Region features encoded by CLIP visual encoder
# x: input image
# targets: ground truth annotations (bounding boxes and labels)
# query_embeds: learnable queries 

# annotations
gt_boxes, gt_labels = targets['boxes'], targets['labels']

# Forward pass to get predictions
srcs = f(x)  # Extract features
hs = transformer(srcs, query_embeds, semantic_features[gt_labels])  # Transformer encoder decoder pass

# Generate predictions
pred_boxes = bbox_head(hs)  # Predicted bounding boxes
pred_embeds = feature_head(hs)  # Predicted class logits

# Hungarian matching
indices = hungarian_matcher(pred_boxes, pred_embeds, gt_boxes, semantic_features[:])

# Calculate loss
loss = 0
for (pred_idx, gt_idx) in indices:
    bbox_loss = L1(pred_boxes[pred_idx], gt_boxes[gt_idx]) + GiOU(pred_boxes[pred_idx], gt_boxes[gt_idx])
    
    similarity_score = cosine(pred_embeds, regional_guidance[gt_labels].T) / temperature
    target_positives_map = torch.zeros([similarity_score.shape])
    target_positives_map.scatter_(1, gt_labels[gt_idx])
    feat_loss = Contras(similarity_score, target_positives_map)
    
    loss += feat_loss + bbox_loss
\end{lstlisting}
